# Supplementary material for: Estimation of Evaporator Valve Sizes in Supermarket Refrigeration Cabinets
Source: arXiv:2202.10348 source file (2022-02-21)
Supplement: Supplementary file 1 [file structure.tex]

\newpage
\section{Cabinet structure}\label{Appendix:structure}
\begin{figure*}
	\centering
		\includegraphics[scale=0.8, angle =-90 ]{Figures/Fakta Otterup Rørdiagram med Pos numre.pdf}
	\caption{Cabinet system structure}
	\label{fig:structure}
\end{figure*}
